# Supplementary material for: Explainable Human-AI Interaction: A Planning Perspective
Source: arXiv:2405.15804 source file (2024-05-19)
Supplement: Supplementary file 1 [file appendix1.tex]

\chapter{Code}
